# Supplementary material for: Robust Pipek-Mezey Orbital Localization in Periodic Solids
Source: arXiv:2103.04562 source file (2021-07-16)
Supplement: Supplementary file 1 [file supp-info.pdf]

# Supporting Information for "Robust Pipek-Mezey Orbital Localization in Periodic Solids"

Marjory C. Clement,† Xiao Wang,†,‡ and Edward F. Valeev*,†

†*Department of Chemistry, Virginia Tech, Blacksburg, VA 24061*

‡*Center for Computational Quantum Physics, Flatiron Institute, New York, New York 10010, USA*

E-mail: efv@vt.edu

## I Input Files

To enable reproducibility of the data reported in the manuscript, complete input files for all test systems considered in this work, in plain text format, can be found in the accompanying `inputs.zip` file. The archive includes a single input file for each system (in JSON format, along with the corresponding XYZ file specifying the Cartesian geometries of the atoms) specifying the $\langle 2, 15\rangle$ BFGS solver. In the following tables, we explain in detail what each of the pertinent `Keys` are and the possible `Vals` that can be assigned to them. Possible values are broken down by solver class (BFGS, CG, SA) to allow the reader to recreate any of the calculations reported in the current work.

We have also summarized how to achieve each of the different initial guess scenarios, described more in Section IV.

Table 1: Each of the pertinent `Keys`, along with their description

| `Key` | Description |
|---|---|
| `"convergence"` | Error norm convergence threshold |
| `"max_iter"` | Max iters solver is allowed |
| `"initial_W"` | The initial estimate for the $\{\mathbf{U_k}\}$ |
| `"duplicate_W"` | Whether or not to use the same pseudorandom unitary matrix for each $\mathbf{k}$ point |
| `"seed"` | The seed to generate pseudorandom unitary matrices. Note: A seed of 0.0 will use the current time as the seed |
| `"iters_kept"` | The history size |
| `"bfgs_start"` | The no. of SA steps to perform initially |
| `"charge_exponent"` | The PM functional exponent |
| `"solver"` | The solver class |

Table 2: For each `Key`, the possible values, broken down by solver type

| `Key` | BFGS values | CG values | SA values |
|---|---|---|---|
| `"convergence"` | double | double | double |
| `"max_iter"` | int | int | int |
| `"initial_W"` | `"identity"`, `"random"` | `"identity"`, `"random"` | `"identity"`, `"random"` |
| `"duplicate_W"` | `true`, `false` | `true`, `false` | `true`, `false` |
| `"seed"` | double | double | double |
| `"iters_kept"` | int | n/a | n/a |
| `"bfgs_start"` | int | int | n/a |
| `"charge_exponent"` | 2, 4 | 2, 4 | 2, 4 |
| `"solver"` | `"bfgs"` | `"cgpr"`, `"cgfr"`, `"cghs"` | `"sa"` |

Table 3: The pertinent `Keys` and associated `Vals` for choosing each of the different initial guess scenarios

| Initial guess | `"initial_W"` | `"duplicate_W"` | `"seed"` |
|---|---|---|---|
| CPR | `"random"` | `true` | double |
| CP | `"identity"` | n/a | n/a |
| Random | `"random"` | `false` | double |

# II PM Functional Values Obtained with Different Solvers

For each system and solver class, we have determined the minimum, maximum, and mean final PM functional values, along with the standard deviation. Calculations that failed to

converge in $4,000$ iterations were excluded, though only when all calculations in a particular solver class failed to converge is this noted in this document. More details about the number and type of calculations that failed to converge can be found in the footnotes to Table 2 in the main text.

Table 4: $P$ Value Summary

| System | Solver | Min | Max | Mean | St. Dev. |
|---|---|---|---|---|---|
| trans-$(C_2H_2)_\infty$ | L-BFGS | 4.56799 | 4.56799 | 4.56799 | $1.28433 \times 10^{-12}$ |
| | CG | 4.56799 | 4.56799 | 4.56799 | $2.24573 \times 10^{-12}$ |
| | CGPR | 4.56799 | 4.56799 | 4.56799 | $6.66975 \times 10^{-13}$ |
| | CGFR | 4.56799 | 4.56799 | 4.56799 | $1.63555 \times 10^{-12}$ |
| | CGHS | 4.56799 | 4.56799 | 4.56799 | $7.75747 \times 10^{-13}$ |
| $(C_2H_4)_\infty$ | L-BFGS | 5.12161 | 5.12161 | 5.12161 | $9.31529 \times 10^{-15}$ |
| | CG | 5.12161 | 5.12161 | 5.12161 | $6.96696 \times 10^{-13}$ |
| | CGPR | 5.12161 | 5.12161 | 5.12161 | $1.00829 \times 10^{-12}$ |
| | CGFR | 5.12161 | 5.12161 | 5.12161 | $7.07957 \times 10^{-14}$ |
| | CGHS | 5.12161 | 5.12161 | 5.12161 | $6.02599 \times 10^{-13}$ |
| (4,0) nanotube | L-BFGS | 31.19107 | 31.19176 | 31.19167 | $1.93878 \times 10^{-4}$ |
| | CG | 31.19107 | 31.19176 | 31.19169 | $1.98526 \times 10^{-4}$ |
| | CGPR | 31.19176 | 31.19176 | 31.19176 | $9.44383 \times 10^{-11}$ |
| | CGFR | 31.19107 | 31.19176 | 31.19154 | $3.14052 \times 10^{-4}$ |
| | CGHS | 31.19176 | 31.19176 | 31.19176 | $8.10078 \times 10^{-12}$ |
| Graphene | L-BFGS | 3.89326 | 3.89326 | 3.89326 | $7.04501 \times 10^{-11}$ |
| | CG | 3.89326 | 3.89326 | 3.89326 | $4.48737 \times 10^{-10}$ |
| | CGPR | 3.89326 | 3.89326 | 3.89326 | $4.93482 \times 10^{-10}$ |
| | CGFR | 3.89326 | 3.89326 | 3.89326 | $8.32480 \times 10^{-11}$ |
| | CGHS[a] | – | – | – | – |
| h-BN | L-BFGS | 8.25633 | 8.25633 | 8.25633 | $9.34466 \times 10^{-13}$ |
| | CG | 8.25633 | 8.25633 | 8.25633 | $3.82389 \times 10^{-12}$ |
| | CGPR | 8.25633 | 8.25633 | 8.25633 | $2.21896 \times 10^{-12}$ |
| | CGFR | 8.25633 | 8.25633 | 8.25633 | $9.41174 \times 10^{-13}$ |
| | CGHS | 8.25633 | 8.25633 | 8.25633 | $1.06368 \times 10^{-12}$ |
| LiH | L-BFGS | 1.69834 | 1.69834 | 1.69834 | $1.36862 \times 10^{-13}$ |
| | CG | 1.69834 | 1.69834 | 1.69834 | $1.51313 \times 10^{-9}$ |
| | CGPR | 1.69834 | 1.69834 | 1.69834 | $1.09185 \times 10^{-9}$ |
| | CGFR | 1.69834 | 1.69834 | 1.69834 | $8.55046 \times 10^{-13}$ |
| | CGHS | 1.69834 | 1.69834 | 1.69834 | $6.92907 \times 10^{-10}$ |
| Diamond | L-BFGS | 4.13437 | 4.13437 | 4.13437 | $1.82115 \times 10^{-12}$ |
| | CG | 4.13437 | 4.13437 | 4.13437 | $2.66713 \times 10^{-12}$ |
| | CGPR | 4.13437 | 4.13437 | 4.13437 | $2.22468 \times 10^{-12}$ |
| | CGFR | 4.13437 | 4.13437 | 4.13437 | $3.01420 \times 10^{-12}$ |
| | CGHS[a] | – | – | – | – |
| Silicon | L-BFGS | 12.17338 | 12.17338 | 12.17338 | $1.20008 \times 10^{-6}$ |
| | CG | 12.17338 | 12.17338 | 12.17338 | $7.02816 \times 10^{-7}$ |
| | CGPR | 12.17338 | 12.17338 | 12.17338 | $1.70569 \times 10^{-7}$ |
| | CGFR | 12.17338 | 12.17338 | 12.17338 | $9.91283 \times 10^{-8}$ |
| | CGHS | 12.17338 | 12.17338 | 12.17338 | $2.38640 \times 10^{-7}$ |

[a] All five calculations failed to converge.

# III Number of Iterations to Solution vs. BFGS Parameters

For each system, we have tabulated the number of iterations to solution for every BFGS solver; this data is organized by BFGS parameter pair. This should allow the interested reader to recreate the analysis in Table 3 of the manuscript.

Table 5: The number of iterations to solution for every parameter pair of the BFGS solver.

| ⟨ # of SA, History ⟩ | trans-$(C_2H_2)_\infty$ | $(C_2H_4)_\infty$ | (4,0) nanotube | Graphene | h-BN | LiH | Diamond | Silicon |
|---|---|---|---|---|---|---|---|---|
| ⟨1, 1⟩ | 40 | 24 | 96 | 150 | 50 | 10 | 23 | 24 |
| ⟨1, 2⟩ | 31 | 26 | 101 | 96 | 49 | 11 | 24 | 22 |
| ⟨1, 5⟩ | 38 | 26 | 98 | 72 | 57 | 11 | 24 | 27 |
| ⟨1, 10⟩ | 44 | 27 | 95 | 55 | 56 | 11 | 24 | 28 |
| ⟨1, 15⟩ | 38 | 27 | 98 | 54 | 56 | 11 | 25 | 29 |
| ⟨2, 1⟩ | 40 | 26 | 98 | 186 | 52 | 10 | 23 | 21 |
| ⟨2, 2⟩ | 37 | 26 | 93 | 76 | 47 | 11 | 23 | 23 |
| ⟨2, 5⟩ | 38 | 26 | 86 | 63 | 51 | 11 | 24 | 25 |
| ⟨2, 10⟩ | 44 | 27 | 92 | 55 | 50 | 11 | 24 | 23 |
| ⟨2, 15⟩ | 37 | 27 | 87 | 54 | 50 | 11 | 25 | 23 |
| ⟨5, 1⟩ | 41 | 30 | 77 | 180 | 56 | 12 | 23 | 22 |
| ⟨5, 2⟩ | 38 | 27 | 76 | 109 | 52 | 12 | 23 | 22 |
| ⟨5, 5⟩ | 39 | 27 | 78 | 75 | 51 | 13 | 24 | 22 |
| ⟨5, 10⟩ | 44 | 28 | 81 | 56 | 51 | 13 | 25 | 24 |
| ⟨5, 15⟩ | 38 | 29 | 80 | 54 | 51 | 13 | 25 | 25 |
| ⟨10, 1⟩ | 45 | 30 | 78 | 86 | 45 | 17 | 24 | 22 |
| ⟨10, 2⟩ | 39 | 31 | 75 | 100 | 47 | 17 | 24 | 23 |
| ⟨10, 5⟩ | 46 | 31 | 77 | 53 | 45 | 17 | 25 | 23 |
| ⟨10, 10⟩ | 45 | 31 | 82 | 54 | 48 | 17 | 25 | 24 |
| ⟨10, 15⟩ | 41 | 32 | 80 | 55 | 48 | 18 | 27 | 25 |
| ⟨15, 1⟩ | 47 | 37 | 93 | 160 | 47 | 21 | 27 | 25 |
| ⟨15, 2⟩ | 41 | 34 | 83 | 122 | 50 | 21 | 26 | 24 |
| ⟨15, 5⟩ | 40 | 32 | 81 | 74 | 48 | 21 | 26 | 25 |
| ⟨15, 10⟩ | 41 | 32 | 83 | 56 | 49 | 21 | 27 | 25 |
| ⟨15, 15⟩ | 41 | 33 | 85 | 56 | 50 | 22 | 28 | 26 |

# IV Initial Guess

To probe the sensitivity of the solver to the initial guess, the $\langle 2, 15\rangle$ BFGS PM solver was run on trans-$(C_2H_2)_\infty$ with 25 different initial guess scenarios:

1. 12 calculations using the CPR guess, each with a different seed.

2. 1 calculation using the "CP" guess (CPR without Randomization), in which, after phase canonicalization, an identity matrix was used to initialize every $\mathbf{U_k}$ matrix.

3. 12 calculations where each $\mathbf{U_k}$ matrix was initialized with a different seed.

Scenario (1) is what was used throughout the main text. Clearly, the phase canonicalization used in scenarios (1) and (2) leads to much greater starting values of $P$, thereby requiring fewer iterations to converge. The "$\mathbf{k}$-nonuniform" random guesses [scenario (3)] were of much lower quality (smaller value of $P$) and resulted in slower convergence. However, the final value of $P$ was the same, irrespective of the initial guess.

Table 6: A statistical analysis of initial $P$, final $P$, and the number of iterations to solution vs. the initial guess type

| | | Min | Max | Mean | St. Dev. |
|---|---|---|---|---|---|
| | Initial $P$ | 1.20267281 | 1.35176477 | 1.27035531 | $4.81965353 \times 10^{-2}$ |
| CPR | Final $P$ | 4.56798693 | 4.56798693 | 4.56798693 | $1.48958067 \times 10^{-14}$ |
| | No. iters | 37 | 42 | 39.2 | 1.90 |
| | Initial $P$ | 1.23188514 | – | – | – |
| CP | Final $P$ | 4.56798693 | – | – | – |
| | No. iters | 37 | – | – | – |
| | Initial $P$ | 0.17368364 | 0.19225600 | 0.18193346 | $6.26283073 \times 10^{-3}$ |
| Random | Final $P$ | 4.56798693 | 4.56798693 | 4.56798693 | $4.09819998 \times 10^{-13}$ |
| | No. iters | 67 | 82 | 75.2 | 4.69 |

# V Minimal Basis Set Choice

We are also interested in how sensitive the solver is to the choice of minimal basis set used to compute the atomic charges. To this end, we have tabulated the initial $P$ value, the final $P$ value, and the number of iterations to solution for 16 different calculations. For each of the eight systems studied herein, we ran the $\langle 2, 15 \rangle$ BFGS PM solver twice, once using the Huzinaga MINI basis set[?, ?, ?] for the minimal basis set and once using Knizia's cc-pVTZ-derived MINAO basis.[?] In all cases, the CPR guess with a seed of 1.0 was used.

In all cases, the MINI minimal basis set produced a slightly higher initial $P$ value than did MINAO, and in all but three cases (carbon nanotube, h-BN, and diamond), the MINI-based calculation converged in the same number or fewer iterations than the one that used

the MINAO basis. The final $P$ value was slightly higher for the MINI calculations in all cases except for h-BN and diamond. Though the initial $P$ value is much less sensitive to the choice of the minimal basis than it is to the choice of the initial guess generating logic (CPR vs. CP vs. Random), the final $P$ value varies a fair bit more with the variation in minimal basis than it does with the variation in initial guess logic.

Table 7: Comparison of initial $P$, final $P$, and the number of iterations to solution vs. the minimal basis set employed

| System | Minimal Basis | Initial $P$ | Final $P$ | No. iters |
|---|---|---|---|---|
| trans-$(C_2H_2)_\infty$ | MINI | 1.35176 | 4.56799 | 37 |
| | MINAO | 1.34997 | 4.55664 | 38 |
| $(C_2H_4)_\infty$ | MINI | 1.65401 | 5.12161 | 27 |
| | MINAO | 1.64906 | 5.12157 | 27 |
| (4,0) nanotube | MINI | 1.99298 | 31.19176 | 87 |
| | MINAO | 1.98765 | 31.17120 | 84 |
| Graphene | MINI | 1.26844 | 3.89326 | 54 |
| | MINAO | 1.25791 | 3.88672 | 65 |
| h-BN | MINI | 1.06602 | 8.25633 | 50 |
| | MINAO | 1.06308 | 8.28429 | 47 |
| LiH | MINI | 0.93803 | 1.69834 | 11 |
| | MINAO | 0.89262 | 1.69277 | 11 |
| Diamond | MINI | 0.63132 | 4.13437 | 25 |
| | MINAO | 0.62478 | 4.14208 | 24 |
| Silicon | MINI | 1.39184 | 12.17338 | 23 |
| | MINAO | 1.38606 | 12.08619 | 24 |

In looking at Table 7, we see that LiH had the largest difference in initial $P$ value (though only the second smallest absolute difference in final $P$ value) with variation in the minimal basis. This led us to explore how the BFGS solver as applied to LiH would respond to the use of other minimal bases. In particular, we employed STO-3G and a variant of the MINAO basis where we maintained the $2p$ orbitals on Li found in the cc-pVTZ basis set[?, ?] (we are calling this "MINAO w/ $2p$"). We compare the maximum overlap condition number, the initial $P$ value, the final $P$ value, and the number of iterations to solution for the four minimal bases (MINI, MINAO, MINAO w/ $2p$, and STO-3G). This data can be found in

Table 8. The presence of the unoccupied valence $p$ orbital, far more than the maximum overlap condition number, seems to be the indicator of poor BFGS convergence behavior.

Table 8: Comparison of maximum overlap condition number, initial $P$, final $P$, and the number of iterations to solution vs. the minimal basis set employed

| Minimal Basis | Max Condition Number | Initial $P$ | Final $P$ | No. iters |
|---|---|---|---|---|
| STO-3G | 114.53596 | 0.84045 | 1.21610 | 20 |
| MINAO w/ 2$p$ | 3233.44358 | 0.73236 | 1.27476 | 19 |
| MINAO | 96.46795 | 0.89262 | 1.69277 | 11 |
| MINI | 102.88753 | 0.93803 | 1.69834 | 11 |
